# Supplementary material for: New measurement of $\theta_{13}$ via neutron capture on hydrogen at Daya Bay
Source: arXiv:1603.03549 source file (2016-04-25)
Supplement: Supplementary file 1 [file SupplementalMaterial.pdf]

# Daya Bay Reactor Neutrino Experiment

## Supplemental Material

March 2016

This document provides supplemental information that is necessary to reproduce the determination of $\sin^2 2\theta_{13} = 0.071 \pm 0.011$ in the article "New measurement of $\theta_{13}$ via neutron capture on hydrogen at Daya Bay".

**CONTENTS**

I. TARGET PROTONS 2

II. EFFICIENCY-WEIGHTED TARGET PROTONS 2

III. BASELINES 2

IV. EFFICIENCY CORRECTION FACTORS 3

V. IBD FRACTIONS 5

VI. PREDICTED REACTOR ANTINEUTRINO SPECTRA 6

# I. TARGET PROTONS

Table I lists the masses $M$ and number of target protons $N_p$ of the GdLS, LS, and acrylic volumes of each antineutrino detector (AD). The calculation of $N_p$ followed Eq. (23) of the main text and used H mass fractions of 12.0%, 12.0%, and 8.05%, Avogadro's number (6.022141E23 mol$^{-1}$), and the molar mass of hydrogen (1.007975 g mol$^{-1}$).

| Detector | $M_{\rm LS}$ | $N_{p,\rm LS}$ | $M_{\rm GdLS}$ | $N_{p,\rm GdLS}$ | $M_{\rm acrylic}$ | $N_{p,\rm acrylic}$ |
|---|---|---|---|---|---|---|
| EH1-AD1 | 21574 | 1.547e+30 | 19941 | 1.430e+30 | 3697 | 0.178e+30 |
| EH1-AD2 | 21520 | 1.543e+30 | 19967 | 1.431e+30 | 3731 | 0.179e+30 |
| EH2-AD1 | 21587 | 1.548e+30 | 19891 | 1.426e+30 | 3664 | 0.176e+30 |
| EH2-AD2 | 21450 | 1.538e+30 | 19944 | 1.430e+30 | 3749 | 0.180e+30 |
| EH3-AD1 | 21566 | 1.546e+30 | 19917 | 1.428e+30 | 3744 | 0.180e+30 |
| EH3-AD2 | 21409 | 1.535e+30 | 19989 | 1.433e+30 | 3864 | 0.186e+30 |
| EH3-AD3 | 21653 | 1.553e+30 | 19892 | 1.426e+30 | 3844 | 0.185e+30 |
| EH3-AD4 | 21475 | 1.540e+30 | 19931 | 1.429e+30 | 3794 | 0.183e+30 |

TABLE I. Masses [kg] and number of target protons of the GdLS, LS, and acrylic volumes of each AD.

# II. EFFICIENCY-WEIGHTED TARGET PROTONS

Table II lists the efficiency-weighted number of target protons for the LS, GdLS, and acrylic volumes of each AD. The calculation of these numbers followed Eq. (12) of the main text such that the sum of the values of each volume equals $N_\varepsilon$: $N_{\varepsilon,\rm LS} + N_{\varepsilon,\rm GdLS} + N_{\varepsilon,\rm acrylic} = N_\varepsilon$.

| Detector | $N_{\varepsilon,\rm LS}$ | $N_{\varepsilon,\rm GdLS}$ | $N_{\varepsilon,\rm acrylic}$ |
|---|---|---|---|
| EH1-AD1 | 0.4574e+30 | 0.1151e+30 | 0.0057e+30 |
| EH1-AD2 | 0.4546e+30 | 0.1148e+30 | 0.0058e+30 |
| EH2-AD1 | 0.4799e+30 | 0.1203e+30 | 0.0060e+30 |
| EH2-AD2 | 0.4768e+30 | 0.1207e+30 | 0.0061e+30 |
| EH3-AD1 | 0.5643e+30 | 0.1419e+30 | 0.0072e+30 |
| EH3-AD2 | 0.5601e+30 | 0.1423e+30 | 0.0074e+30 |
| EH3-AD3 | 0.5665e+30 | 0.1416e+30 | 0.0074e+30 |
| EH3-AD4 | 0.5622e+30 | 0.1420e+30 | 0.0073e+30 |

TABLE II. Efficiency-weighted number of target protons of each volume of each AD.

# III. BASELINES

Table III lists the baseline distances from the centers of the eight ADs to the centers of the six nuclear reactor cores. The baselines are introduced as $L_{dr}$ in Section III of the main text.

| Detector | $L_{d1}$ | $L_{d2}$ | $L_{d3}$ | $L_{d4}$ | $L_{d5}$ | $L_{d6}$ |
|---|---|---|---|---|---|---|
| EH1-AD1 | 362.380 | 371.763 | 903.466 | 817.158 | 1353.618 | 1265.315 |
| EH1-AD2 | 357.940 | 368.414 | 903.347 | 816.896 | 1354.229 | 1265.886 |
| EH2-AD1 | 1332.479 | 1358.148 | 467.574 | 489.577 | 557.579 | 499.207 |
| EH2-AD2 | 1337.429 | 1362.876 | 472.971 | 495.346 | 558.707 | 501.071 |
| EH3-AD1 | 1919.632 | 1894.338 | 1533.180 | 1533.628 | 1551.384 | 1524.940 |
| EH3-AD2 | 1917.519 | 1891.977 | 1534.919 | 1535.032 | 1554.767 | 1528.046 |
| EH3-AD3 | 1925.255 | 1899.861 | 1538.930 | 1539.468 | 1556.344 | 1530.079 |
| EH3-AD4 | 1923.149 | 1897.507 | 1540.667 | 1540.872 | 1559.721 | 1533.179 |

TABLE III. Baselines [meter] between each AD and reactor core.

## IV. EFFICIENCY CORRECTION FACTORS

This section provides the efficiency correction factors described in Section VII.1.1 of the main text. Factors were calculated for each fit iteration. The factors supplied in Tables IV-IX were calculated after the third fit (used for the fourth fit).

The three sets of factors listed in Tables IV, V, and VI were generated assuming the normal neutrino mass hierarchy. The three sets of factors listed in Tables VII, VIII, and IX were generated assuming the inverted neutrino mass hierarchy.

| Detector | Reactor 1 | Reactor 2 | Reactor 3 | Reactor 4 | Reactor 5 | Reactor 6 |
|---|---|---|---|---|---|---|
| EH1-AD1 | 1.00052 | 1.00077 | 1.00210 | 1.00181 | 1.00028 | 1.00138 |
| EH1-AD2 | 1.00053 | 1.00092 | 1.00208 | 1.00216 | 1.00108 | 1.00149 |
| EH2-AD1 | 1.00093 | 1.00061 | 1.00109 | 1.00122 | 1.00162 | 1.00127 |
| EH2-AD2 | 1.00086 | 1.00074 | 1.00103 | 1.00101 | 1.00138 | 1.00098 |
| EH3-AD1 | 0.99731 | 0.99727 | 0.99964 | 0.99939 | 0.99934 | 0.99989 |
| EH3-AD2 | 0.99711 | 0.99794 | 0.99968 | 0.99978 | 0.99935 | 1.00010 |
| EH3-AD3 | 0.99753 | 0.99783 | 1.00016 | 0.99982 | 0.99978 | 1.00014 |
| EH3-AD4 | 0.99684 | 0.99768 | 0.99970 | 0.99907 | 0.99933 | 0.99968 |

TABLE IV. Efficiency correction factors for the LS volume of each detector-reactor pair assuming the normal mass hierarchy.

| Detector | Reactor 1 | Reactor 2 | Reactor 3 | Reactor 4 | Reactor 5 | Reactor 6 |
|---|---|---|---|---|---|---|
| EH1-AD1 | 1.00084 | 1.00032 | 1.00144 | 1.00190 | 1.00038 | 1.00180 |
| EH1-AD2 | 1.00070 | 1.00028 | 1.00066 | 1.00039 | 1.00033 | 1.00145 |
| EH2-AD1 | 0.99941 | 0.99994 | 1.00013 | 1.00095 | 1.00177 | 1.00103 |
| EH2-AD2 | 1.00067 | 0.99998 | 1.00121 | 1.00087 | 1.00117 | 1.00115 |
| EH3-AD1 | 0.99837 | 0.99693 | 0.99982 | 0.99912 | 0.99775 | 0.99797 |
| EH3-AD2 | 0.99698 | 0.99756 | 1.00047 | 1.00055 | 1.00047 | 0.99984 |
| EH3-AD3 | 0.99815 | 0.99842 | 0.99921 | 0.99937 | 0.99972 | 0.99972 |
| EH3-AD4 | 0.99675 | 0.99805 | 0.99973 | 1.00120 | 0.99812 | 0.99887 |

TABLE V. Efficiency correction factors for the GdLS volume of each detector-reactor pair assuming the normal mass hierarchy.

| Detector | Reactor 1 | Reactor 2 | Reactor 3 | Reactor 4 | Reactor 5 | Reactor 6 |
|---|---|---|---|---|---|---|
| EH1-AD1 | 1.00199 | 1.00192 | 1.00443 | 1.00672 | 1.00573 | 1.00264 |
| EH1-AD2 | 1.00152 | 1.00122 | 1.00296 | 1.00472 | 1.00830 | 1.00643 |
| EH2-AD1 | 1.00130 | 1.00111 | 1.00211 | 1.00037 | 0.99951 | 1.00017 |
| EH2-AD2 | 1.00389 | 1.00222 | 1.00381 | 1.00103 | 1.00116 | 1.00019 |
| EH3-AD1 | 0.99646 | 1.00105 | 1.00351 | 0.99779 | 1.00175 | 1.00236 |
| EH3-AD2 | 0.99930 | 0.99597 | 1.00211 | 1.00201 | 1.00319 | 1.00052 |
| EH3-AD3 | 0.99641 | 0.99435 | 1.00397 | 1.00269 | 1.00571 | 1.00312 |
| EH3-AD4 | 0.99588 | 0.99492 | 0.99899 | 1.00318 | 1.00055 | 1.00456 |

TABLE VI. Efficiency correction factors for the acrylic volume of each detector-reactor pair assuming the normal mass hierarchy.

| Detector | Reactor 1 | Reactor 2 | Reactor 3 | Reactor 4 | Reactor 5 | Reactor 6 |
|---|---|---|---|---|---|---|
| EH1-AD1 | 1.00077 | 1.00085 | 1.00276 | 1.00245 | 1.00118 | 1.00174 |
| EH1-AD2 | 1.00074 | 1.00075 | 1.00247 | 1.00255 | 1.00122 | 1.00181 |
| EH2-AD1 | 1.00116 | 1.00131 | 1.00120 | 1.00122 | 1.00146 | 1.00139 |
| EH2-AD2 | 1.00129 | 1.00124 | 1.00115 | 1.00128 | 1.00173 | 1.00142 |
| EH3-AD1 | 0.99711 | 0.99738 | 0.99989 | 1.00006 | 0.99971 | 1.00013 |
| EH3-AD2 | 0.99712 | 0.99721 | 0.99999 | 0.99983 | 0.99963 | 1.00011 |
| EH3-AD3 | 0.99708 | 0.99722 | 0.99984 | 0.99982 | 0.99977 | 0.99989 |
| EH3-AD4 | 0.99710 | 0.99717 | 1.00000 | 0.99989 | 0.99969 | 0.99998 |

TABLE VII. Efficiency correction factors for the LS volume of each detector-reactor pair assuming the inverted mass hierarchy.

| Detector | Reactor 1 | Reactor 2 | Reactor 3 | Reactor 4 | Reactor 5 | Reactor 6 |
|---|---|---|---|---|---|---|
| EH1-AD1 | 1.00063 | 1.00051 | 1.00191 | 1.00172 | 1.00090 | 1.00093 |
| EH1-AD2 | 1.00054 | 1.00050 | 1.00182 | 1.00169 | 1.00063 | 1.00094 |
| EH2-AD1 | 1.00069 | 1.00074 | 1.00068 | 1.00080 | 1.00098 | 1.00098 |
| EH2-AD2 | 1.00074 | 1.00064 | 1.00091 | 1.00101 | 1.00109 | 1.00090 |
| EH3-AD1 | 0.99761 | 0.99785 | 0.99991 | 0.99969 | 0.99946 | 0.99973 |
| EH3-AD2 | 0.99800 | 0.99797 | 0.99973 | 0.99949 | 0.99927 | 0.99985 |
| EH3-AD3 | 0.99803 | 0.99811 | 0.99993 | 0.99936 | 0.99945 | 0.99989 |
| EH3-AD4 | 0.99780 | 0.99790 | 0.99986 | 0.99959 | 0.99931 | 0.99959 |

TABLE VIII. Efficiency correction factors for the GdLS volume of each detector-reactor pair assuming the inverted mass hierarchy.

| Detector | Reactor 1 | Reactor 2 | Reactor 3 | Reactor 4 | Reactor 5 | Reactor 6 |
|---|---|---|---|---|---|---|
| EH1-AD1 | 1.00037 | 1.00084 | 1.00507 | 1.00310 | 1.00672 | 1.00442 |
| EH1-AD2 | 1.00126 | 1.00090 | 1.00699 | 1.00881 | 1.00606 | 1.00629 |
| EH2-AD1 | 1.00805 | 1.00673 | 1.00201 | 1.00164 | 1.00278 | 1.00081 |
| EH2-AD2 | 1.00736 | 1.00750 | 1.00272 | 1.00259 | 1.00443 | 1.00227 |
| EH3-AD1 | 1.00110 | 0.99921 | 1.00409 | 1.00435 | 1.00418 | 1.00150 |
| EH3-AD2 | 0.99828 | 1.00015 | 1.00165 | 1.00583 | 1.00762 | 1.00569 |
| EH3-AD3 | 0.99665 | 1.00050 | 1.00570 | 1.00420 | 1.00303 | 1.00524 |
| EH3-AD4 | 1.00223 | 0.99546 | 1.00347 | 1.00348 | 1.00335 | 1.00494 |

TABLE IX. Efficiency correction factors for the acrylic volume of each detector-reactor pair assuming the inverted mass hierarchy.

## V. IBD FRACTIONS

Table X lists the predicted fractions of inverse $\beta$-decays (IBDs) in each AD due to each nuclear reactor. These fractions are introduced as $\omega_r^d$ in Eq. (28) of the main text.

| Detector | $\omega_1^d$ | $\omega_2^d$ | $\omega_3^d$ | $\omega_4^d$ | $\omega_5^d$ | $\omega_6^d$ |
|---|---|---|---|---|---|---|
| EH1-AD1 | 0.384 | 0.408 | 0.064 | 0.083 | 0.031 | 0.031 |
| EH1-AD2 | 0.387 | 0.408 | 0.063 | 0.081 | 0.030 | 0.030 |
| EH2-AD1 | 0.032 | 0.034 | 0.262 | 0.254 | 0.198 | 0.220 |
| EH2-AD2 | 0.033 | 0.032 | 0.253 | 0.252 | 0.193 | 0.238 |
| EH3-AD1 | 0.115 | 0.131 | 0.185 | 0.197 | 0.194 | 0.179 |
| EH3-AD2 | 0.115 | 0.132 | 0.185 | 0.197 | 0.194 | 0.178 |
| EH3-AD3 | 0.115 | 0.131 | 0.185 | 0.196 | 0.194 | 0.179 |
| EH3-AD4 | 0.122 | 0.123 | 0.180 | 0.196 | 0.186 | 0.192 |

TABLE X. Predicted fractions of IBDs in each AD due to each nuclear reactor.

## VI. PREDICTED REACTOR ANTINEUTRINO SPECTRA

Tables XI-XV provide the predicted reactor antineutrino energy spectrum from each nuclear reactor integrated over the data acquisition periods of each AD [$dN_r(E)/dE$ from Eq. (2) of the main text]. Because EH2-AD2 and EH3-AD4 were installed after the other six ADs, they have distinct predicted spectra given in Tables XIII and XV, respectively.

| Energy [MeV] | Reactor 1 | Reactor 2 | Reactor 3 | Reactor 4 | Reactor 5 | Reactor 6 |
|---|---|---|---|---|---|---|
| ( 1.375, 1.625 ) | 6.1430e+27 | 6.7985e+27 | 6.2797e+27 | 6.7112e+27 | 6.7924e+27 | 6.0289e+27 |
| ( 1.625, 1.875 ) | 5.4706e+27 | 6.0584e+27 | 5.5882e+27 | 5.9682e+27 | 6.0418e+27 | 5.3642e+27 |
| ( 1.875, 2.125 ) | 4.6443e+27 | 5.1401e+27 | 4.7425e+27 | 5.0664e+27 | 5.1278e+27 | 4.5526e+27 |
| ( 2.125, 2.375 ) | 3.9433e+27 | 4.3614e+27 | 4.0253e+27 | 4.3013e+27 | 4.3526e+27 | 3.8643e+27 |
| ( 2.375, 2.625 ) | 3.1962e+27 | 3.5400e+27 | 3.2655e+27 | 3.4875e+27 | 3.5283e+27 | 3.1319e+27 |
| ( 2.625, 2.875 ) | 2.6949e+27 | 2.9797e+27 | 2.7516e+27 | 2.9412e+27 | 2.9743e+27 | 2.6398e+27 |
| ( 2.875, 3.125 ) | 2.2495e+27 | 2.4898e+27 | 2.2988e+27 | 2.4566e+27 | 2.4851e+27 | 2.2055e+27 |
| ( 3.125, 3.375 ) | 1.8608e+27 | 2.0685e+27 | 1.9068e+27 | 2.0343e+27 | 2.0583e+27 | 1.8261e+27 |
| ( 3.375, 3.625 ) | 1.5304e+27 | 1.7008e+27 | 1.5682e+27 | 1.6734e+27 | 1.6932e+27 | 1.5022e+27 |
| ( 3.625, 3.875 ) | 1.2270e+27 | 1.3641e+27 | 1.2575e+27 | 1.3416e+27 | 1.3579e+27 | 1.2048e+27 |
| ( 3.875, 4.125 ) | 9.7573e+26 | 1.0878e+27 | 1.0017e+27 | 1.0676e+27 | 1.0803e+27 | 9.5821e+26 |
| ( 4.125, 4.375 ) | 7.7159e+26 | 8.5915e+26 | 7.9149e+26 | 8.4398e+26 | 8.5411e+26 | 7.5770e+26 |
| ( 4.375, 4.625 ) | 5.9061e+26 | 6.5992e+26 | 6.0704e+26 | 6.4643e+26 | 6.5446e+26 | 5.8050e+26 |
| ( 4.625, 4.875 ) | 4.5187e+26 | 5.0589e+26 | 4.6495e+26 | 4.9474e+26 | 5.0105e+26 | 4.4441e+26 |
| ( 4.875, 5.125 ) | 3.5320e+26 | 3.9674e+26 | 3.6413e+26 | 3.8695e+26 | 3.9201e+26 | 3.4762e+26 |
| ( 5.125, 5.375 ) | 2.7699e+26 | 3.1122e+26 | 2.8559e+26 | 3.0346e+26 | 3.0751e+26 | 2.7272e+26 |
| ( 5.375, 5.625 ) | 2.0710e+26 | 2.3283e+26 | 2.1360e+26 | 2.2691e+26 | 2.2995e+26 | 2.0393e+26 |
| ( 5.625, 5.875 ) | 1.6337e+26 | 1.8361e+26 | 1.6845e+26 | 1.7896e+26 | 1.8151e+26 | 1.6103e+26 |
| ( 5.875, 6.125 ) | 1.2040e+26 | 1.3610e+26 | 1.2457e+26 | 1.3204e+26 | 1.3397e+26 | 1.1880e+26 |
| ( 6.125, 6.375 ) | 8.6945e+25 | 9.8772e+25 | 9.0197e+25 | 9.5417e+25 | 9.6961e+25 | 8.5996e+25 |
| ( 6.375, 6.625 ) | 6.6261e+25 | 7.5168e+25 | 6.8684e+25 | 7.2701e+25 | 7.3853e+25 | 6.5501e+25 |
| ( 6.625, 6.875 ) | 4.9347e+25 | 5.5975e+25 | 5.1143e+25 | 5.4136e+25 | 5.5022e+25 | 4.8810e+25 |
| ( 6.875, 7.125 ) | 3.4615e+25 | 3.9345e+25 | 3.5919e+25 | 3.7991e+25 | 3.8612e+25 | 3.4247e+25 |
| ( 7.125, 7.375 ) | 2.2111e+25 | 2.5113e+25 | 2.2929e+25 | 2.4258e+25 | 2.4677e+25 | 2.1897e+25 |
| ( 7.375, 7.625 ) | 1.4136e+25 | 1.6094e+25 | 1.4680e+25 | 1.5517e+25 | 1.5785e+25 | 1.4003e+25 |
| ( 7.625, 7.875 ) | 8.6923e+24 | 9.9942e+24 | 9.0788e+24 | 9.5595e+24 | 9.7310e+24 | 8.6272e+24 |
| ( 7.875, 8.125 ) | 5.0610e+24 | 5.7698e+24 | 5.2593e+24 | 5.5568e+24 | 5.6509e+24 | 5.0122e+24 |
| ( 8.125, 8.375 ) | 2.9719e+24 | 3.3571e+24 | 3.0714e+24 | 3.2572e+24 | 3.3092e+24 | 2.9367e+24 |
| ( 8.375, 8.625 ) | 1.7610e+24 | 1.9699e+24 | 1.8094e+24 | 1.9264e+24 | 1.9554e+24 | 1.7363e+24 |
| ( 8.625, 8.875 ) | 1.0534e+24 | 1.1664e+24 | 1.0758e+24 | 1.1501e+24 | 1.1664e+24 | 1.0364e+24 |
| ( 8.875, 9.125 ) | 6.3641e+23 | 6.9722e+23 | 6.4587e+23 | 6.9337e+23 | 7.0266e+23 | 6.2480e+23 |
| ( 9.125, 9.375 ) | 3.8833e+23 | 4.2087e+23 | 3.9159e+23 | 4.2220e+23 | 4.2757e+23 | 3.8049e+23 |
| ( 9.375, 9.625 ) | 2.3934e+23 | 2.5659e+23 | 2.3981e+23 | 2.5966e+23 | 2.6281e+23 | 2.3406e+23 |

TABLE XI. Predicted reactor antineutrino energy spectrum from each nuclear reactor integrated over the data acquisition time of EH1 (2011/12/24-2013/11/27). Applicable to both ADs in EH1. The energy bins are presented as lower and upper bin edges.

| Energy [MeV] | Reactor 1 | Reactor 2 | Reactor 3 | Reactor 4 | Reactor 5 | Reactor 6 |
|---|---|---|---|---|---|---|
| ( 1.375, 1.625 ) | 6.1978e+27 | 6.8296e+27 | 6.3071e+27 | 6.7450e+27 | 6.8158e+27 | 6.0761e+27 |
| ( 1.625, 1.875 ) | 5.5195e+27 | 6.0860e+27 | 5.6125e+27 | 5.9983e+27 | 6.0627e+27 | 5.4061e+27 |
| ( 1.875, 2.125 ) | 4.6858e+27 | 5.1636e+27 | 4.7632e+27 | 5.0919e+27 | 5.1455e+27 | 4.5882e+27 |
| ( 2.125, 2.375 ) | 3.9785e+27 | 4.3813e+27 | 4.0429e+27 | 4.3230e+27 | 4.3675e+27 | 3.8945e+27 |
| ( 2.375, 2.625 ) | 3.2247e+27 | 3.5561e+27 | 3.2797e+27 | 3.5051e+27 | 3.5405e+27 | 3.1563e+27 |
| ( 2.625, 2.875 ) | 2.7189e+27 | 2.9933e+27 | 2.7636e+27 | 2.9560e+27 | 2.9845e+27 | 2.6605e+27 |
| ( 2.875, 3.125 ) | 2.2696e+27 | 2.5011e+27 | 2.3089e+27 | 2.4690e+27 | 2.4936e+27 | 2.2227e+27 |
| ( 3.125, 3.375 ) | 1.8775e+27 | 2.0779e+27 | 1.9150e+27 | 2.0445e+27 | 2.0654e+27 | 1.8404e+27 |
| ( 3.375, 3.625 ) | 1.5441e+27 | 1.7085e+27 | 1.5749e+27 | 1.6817e+27 | 1.6991e+27 | 1.5140e+27 |
| ( 3.625, 3.875 ) | 1.2380e+27 | 1.3703e+27 | 1.2629e+27 | 1.3484e+27 | 1.3626e+27 | 1.2142e+27 |
| ( 3.875, 4.125 ) | 9.8453e+26 | 1.0927e+27 | 1.0059e+27 | 1.0729e+27 | 1.0841e+27 | 9.6570e+26 |
| ( 4.125, 4.375 ) | 7.7854e+26 | 8.6300e+26 | 7.9488e+26 | 8.4820e+26 | 8.5707e+26 | 7.6362e+26 |
| ( 4.375, 4.625 ) | 5.9595e+26 | 6.6285e+26 | 6.0962e+26 | 6.4963e+26 | 6.5674e+26 | 5.8503e+26 |
| ( 4.625, 4.875 ) | 4.5597e+26 | 5.0812e+26 | 4.6691e+26 | 4.9718e+26 | 5.0280e+26 | 4.4788e+26 |
| ( 4.875, 5.125 ) | 3.5642e+26 | 3.9847e+26 | 3.6566e+26 | 3.8886e+26 | 3.9338e+26 | 3.5033e+26 |
| ( 5.125, 5.375 ) | 2.7952e+26 | 3.1258e+26 | 2.8679e+26 | 3.0495e+26 | 3.0859e+26 | 2.7485e+26 |
| ( 5.375, 5.625 ) | 2.0899e+26 | 2.3384e+26 | 2.1449e+26 | 2.2803e+26 | 2.3076e+26 | 2.0552e+26 |
| ( 5.625, 5.875 ) | 1.6487e+26 | 1.8441e+26 | 1.6915e+26 | 1.7984e+26 | 1.8215e+26 | 1.6228e+26 |
| ( 5.875, 6.125 ) | 1.2151e+26 | 1.3668e+26 | 1.2508e+26 | 1.3268e+26 | 1.3444e+26 | 1.1973e+26 |
| ( 6.125, 6.375 ) | 8.7754e+25 | 9.9187e+25 | 9.0562e+25 | 9.5877e+25 | 9.7303e+25 | 8.6666e+25 |
| ( 6.375, 6.625 ) | 6.6876e+25 | 7.5485e+25 | 6.8964e+25 | 7.3052e+25 | 7.4113e+25 | 6.6012e+25 |
| ( 6.625, 6.875 ) | 4.9805e+25 | 5.6211e+25 | 5.1351e+25 | 5.4397e+25 | 5.5216e+25 | 4.9191e+25 |
| ( 6.875, 7.125 ) | 3.4937e+25 | 3.9510e+25 | 3.6065e+25 | 3.8173e+25 | 3.8749e+25 | 3.4514e+25 |
| ( 7.125, 7.375 ) | 2.2317e+25 | 2.5219e+25 | 2.3022e+25 | 2.4375e+25 | 2.4764e+25 | 2.2068e+25 |
| ( 7.375, 7.625 ) | 1.4268e+25 | 1.6161e+25 | 1.4739e+25 | 1.5591e+25 | 1.5841e+25 | 1.4113e+25 |
| ( 7.625, 7.875 ) | 8.7746e+24 | 1.0035e+25 | 9.1143e+24 | 9.6046e+24 | 9.7658e+24 | 8.6944e+24 |
| ( 7.875, 8.125 ) | 5.1083e+24 | 5.7937e+24 | 5.2803e+24 | 5.5834e+24 | 5.6709e+24 | 5.0513e+24 |
| ( 8.125, 8.375 ) | 2.9993e+24 | 3.3715e+24 | 3.0841e+24 | 3.2731e+24 | 3.3208e+24 | 2.9596e+24 |
| ( 8.375, 8.625 ) | 1.7770e+24 | 1.9786e+24 | 1.8171e+24 | 1.9359e+24 | 1.9622e+24 | 1.7499e+24 |
| ( 8.625, 8.875 ) | 1.0629e+24 | 1.1717e+24 | 1.0805e+24 | 1.1559e+24 | 1.1704e+24 | 1.0445e+24 |
| ( 8.875, 9.125 ) | 6.4201e+23 | 7.0051e+23 | 6.4876e+23 | 6.9692e+23 | 7.0505e+23 | 6.2969e+23 |
| ( 9.125, 9.375 ) | 3.9169e+23 | 4.2292e+23 | 3.9340e+23 | 4.2440e+23 | 4.2901e+23 | 3.8347e+23 |
| ( 9.375, 9.625 ) | 2.4137e+23 | 2.5788e+23 | 2.4095e+23 | 2.6103e+23 | 2.6369e+23 | 2.3590e+23 |

TABLE XII. Predicted reactor antineutrino energy spectrum from each nuclear reactor integrated over the data acquisition time of EH2 (2011/12/24-2013/11/27). Applicable to EH2-AD1. The energy bins are presented as lower and upper bin edges.

| Energy [MeV] | Reactor 1 | Reactor 2 | Reactor 3 | Reactor 4 | Reactor 5 | Reactor 6 |
|---|---|---|---|---|---|---|
| ( 1.375, 1.625 ) | 4.4013e+27 | 4.3154e+27 | 4.1376e+27 | 4.5388e+27 | 4.3992e+27 | 4.3732e+27 |
| ( 1.625, 1.875 ) | 3.9203e+27 | 3.8443e+27 | 3.6830e+27 | 4.0356e+27 | 3.9134e+27 | 3.8899e+27 |
| ( 1.875, 2.125 ) | 3.3281e+27 | 3.2624e+27 | 3.1256e+27 | 3.4264e+27 | 3.3211e+27 | 3.3015e+27 |
| ( 2.125, 2.375 ) | 2.8257e+27 | 2.7689e+27 | 2.6529e+27 | 2.9095e+27 | 2.8188e+27 | 2.8024e+27 |
| ( 2.375, 2.625 ) | 2.2899e+27 | 2.2463e+27 | 2.1519e+27 | 2.3581e+27 | 2.2856e+27 | 2.2716e+27 |
| ( 2.625, 2.875 ) | 1.9309e+27 | 1.8921e+27 | 1.8133e+27 | 1.9897e+27 | 1.9262e+27 | 1.9150e+27 |
| ( 2.875, 3.125 ) | 1.6116e+27 | 1.5804e+27 | 1.5147e+27 | 1.6614e+27 | 1.6096e+27 | 1.5999e+27 |
| ( 3.125, 3.375 ) | 1.3326e+27 | 1.3109e+27 | 1.2560e+27 | 1.3741e+27 | 1.3341e+27 | 1.3250e+27 |
| ( 3.375, 3.625 ) | 1.0960e+27 | 1.0779e+27 | 1.0330e+27 | 1.1304e+27 | 1.0974e+27 | 1.0900e+27 |
| ( 3.625, 3.875 ) | 8.7872e+26 | 8.6443e+26 | 8.2830e+26 | 9.0616e+26 | 8.8011e+26 | 8.7408e+26 |
| ( 3.875, 4.125 ) | 6.9859e+26 | 6.8863e+26 | 6.5969e+26 | 7.2048e+26 | 7.0054e+26 | 6.9533e+26 |
| ( 4.125, 4.375 ) | 5.5250e+26 | 5.4413e+26 | 5.2129e+26 | 5.6979e+26 | 5.5374e+26 | 5.4978e+26 |
| ( 4.375, 4.625 ) | 4.2280e+26 | 4.1740e+26 | 3.9974e+26 | 4.3597e+26 | 4.2454e+26 | 4.2121e+26 |
| ( 4.625, 4.875 ) | 3.2344e+26 | 3.1974e+26 | 3.0614e+26 | 3.3347e+26 | 3.2512e+26 | 3.2246e+26 |
| ( 4.875, 5.125 ) | 2.5275e+26 | 2.5044e+26 | 2.3972e+26 | 2.6057e+26 | 2.5450e+26 | 2.5225e+26 |
| ( 5.125, 5.375 ) | 1.9821e+26 | 1.9643e+26 | 1.8802e+26 | 2.0432e+26 | 1.9965e+26 | 1.9788e+26 |
| ( 5.375, 5.625 ) | 1.4819e+26 | 1.4692e+26 | 1.4062e+26 | 1.5276e+26 | 1.4931e+26 | 1.4797e+26 |
| ( 5.625, 5.875 ) | 1.1693e+26 | 1.1587e+26 | 1.1090e+26 | 1.2049e+26 | 1.1784e+26 | 1.1680e+26 |
| ( 5.875, 6.125 ) | 8.6128e+25 | 8.5704e+25 | 8.1983e+25 | 8.8743e+25 | 8.7056e+25 | 8.6189e+25 |
| ( 6.125, 6.375 ) | 6.2182e+25 | 6.2079e+25 | 5.9349e+25 | 6.4033e+25 | 6.3052e+25 | 6.2371e+25 |
| ( 6.375, 6.625 ) | 4.7393e+25 | 4.7269e+25 | 4.5197e+25 | 4.8809e+25 | 4.8015e+25 | 4.7509e+25 |
| ( 6.625, 6.875 ) | 3.5298e+25 | 3.5200e+25 | 3.3655e+25 | 3.6345e+25 | 3.5770e+25 | 3.5396e+25 |
| ( 6.875, 7.125 ) | 2.4755e+25 | 2.4724e+25 | 2.3634e+25 | 2.5490e+25 | 2.5111e+25 | 2.4837e+25 |
| ( 7.125, 7.375 ) | 1.5817e+25 | 1.5784e+25 | 1.5087e+25 | 1.6280e+25 | 1.6045e+25 | 1.5875e+25 |
| ( 7.375, 7.625 ) | 1.0110e+25 | 1.0107e+25 | 9.6580e+24 | 1.0406e+25 | 1.0267e+25 | 1.0153e+25 |
| ( 7.625, 7.875 ) | 6.2112e+24 | 6.2534e+24 | 5.9700e+24 | 6.3920e+24 | 6.3397e+24 | 6.2570e+24 |
| ( 7.875, 8.125 ) | 3.6187e+24 | 3.6216e+24 | 3.4596e+24 | 3.7251e+24 | 3.6766e+24 | 3.6346e+24 |
| ( 8.125, 8.375 ) | 2.1264e+24 | 2.1145e+24 | 2.0212e+24 | 2.1895e+24 | 2.1499e+24 | 2.1291e+24 |
| ( 8.375, 8.625 ) | 1.2610e+24 | 1.2453e+24 | 1.1912e+24 | 1.2987e+24 | 1.2684e+24 | 1.2585e+24 |
| ( 8.625, 8.875 ) | 7.5492e+23 | 7.4021e+23 | 7.0861e+23 | 7.7767e+23 | 7.5535e+23 | 7.5102e+23 |
| ( 8.875, 9.125 ) | 4.5644e+23 | 4.4424e+23 | 4.2561e+23 | 4.7027e+23 | 4.5426e+23 | 4.5260e+23 |
| ( 9.125, 9.375 ) | 2.7876e+23 | 2.6926e+23 | 2.5818e+23 | 2.8724e+23 | 2.7594e+23 | 2.7552e+23 |
| ( 9.375, 9.625 ) | 1.7195e+23 | 1.6485e+23 | 1.5819e+23 | 1.7720e+23 | 1.6932e+23 | 1.6942e+23 |

TABLE XIII. Predicted reactor antineutrino energy spectrum from each nuclear reactor integrated over the data acquisition time of EH2 during the 8-AD period (2012/10/19-2013/11/27). Applicable to EH2-AD2. The energy bins are presented as lower and upper bin edges.

| Energy [MeV] | Reactor 1 | Reactor 2 | Reactor 3 | Reactor 4 | Reactor 5 | Reactor 6 |
|---|---|---|---|---|---|---|
| ( 1.375, 1.625 ) | 6.1167e+27 | 6.7569e+27 | 6.2487e+27 | 6.6749e+27 | 6.7455e+27 | 6.0002e+27 |
| ( 1.625, 1.875 ) | 5.4473e+27 | 6.0213e+27 | 5.5605e+27 | 5.9359e+27 | 6.0001e+27 | 5.3385e+27 |
| ( 1.875, 2.125 ) | 4.6244e+27 | 5.1086e+27 | 4.7191e+27 | 5.0390e+27 | 5.0924e+27 | 4.5309e+27 |
| ( 2.125, 2.375 ) | 3.9263e+27 | 4.3348e+27 | 4.0054e+27 | 4.2780e+27 | 4.3225e+27 | 3.8458e+27 |
| ( 2.375, 2.625 ) | 3.1825e+27 | 3.5183e+27 | 3.2493e+27 | 3.4687e+27 | 3.5040e+27 | 3.1169e+27 |
| ( 2.625, 2.875 ) | 2.6833e+27 | 2.9615e+27 | 2.7380e+27 | 2.9253e+27 | 2.9538e+27 | 2.6272e+27 |
| ( 2.875, 3.125 ) | 2.2398e+27 | 2.4745e+27 | 2.2875e+27 | 2.4433e+27 | 2.4679e+27 | 2.1950e+27 |
| ( 3.125, 3.375 ) | 1.8530e+27 | 2.0557e+27 | 1.8972e+27 | 2.0233e+27 | 2.0441e+27 | 1.8174e+27 |
| ( 3.375, 3.625 ) | 1.5240e+27 | 1.6902e+27 | 1.5603e+27 | 1.6643e+27 | 1.6815e+27 | 1.4951e+27 |
| ( 3.625, 3.875 ) | 1.2218e+27 | 1.3557e+27 | 1.2512e+27 | 1.3343e+27 | 1.3485e+27 | 1.1990e+27 |
| ( 3.875, 4.125 ) | 9.7170e+26 | 1.0810e+27 | 9.9660e+26 | 1.0617e+27 | 1.0728e+27 | 9.5362e+26 |
| ( 4.125, 4.375 ) | 7.6838e+26 | 8.5378e+26 | 7.8750e+26 | 8.3939e+26 | 8.4820e+26 | 7.5407e+26 |
| ( 4.375, 4.625 ) | 5.8820e+26 | 6.5574e+26 | 6.0395e+26 | 6.4289e+26 | 6.4992e+26 | 5.7771e+26 |
| ( 4.625, 4.875 ) | 4.5005e+26 | 5.0266e+26 | 4.6257e+26 | 4.9202e+26 | 4.9757e+26 | 4.4227e+26 |
| ( 4.875, 5.125 ) | 3.5180e+26 | 3.9419e+26 | 3.6225e+26 | 3.8482e+26 | 3.8928e+26 | 3.4594e+26 |
| ( 5.125, 5.375 ) | 2.7590e+26 | 3.0922e+26 | 2.8411e+26 | 3.0178e+26 | 3.0537e+26 | 2.7140e+26 |
| ( 5.375, 5.625 ) | 2.0628e+26 | 2.3133e+26 | 2.1249e+26 | 2.2566e+26 | 2.2835e+26 | 2.0294e+26 |
| ( 5.625, 5.875 ) | 1.6273e+26 | 1.8242e+26 | 1.6757e+26 | 1.7797e+26 | 1.8025e+26 | 1.6025e+26 |
| ( 5.875, 6.125 ) | 1.1994e+26 | 1.3520e+26 | 1.2391e+26 | 1.3131e+26 | 1.3303e+26 | 1.1823e+26 |
| ( 6.125, 6.375 ) | 8.6627e+25 | 9.8112e+25 | 8.9712e+25 | 9.4884e+25 | 9.6282e+25 | 8.5578e+25 |
| ( 6.375, 6.625 ) | 6.6016e+25 | 7.4667e+25 | 6.8317e+25 | 7.2295e+25 | 7.3336e+25 | 6.5183e+25 |
| ( 6.625, 6.875 ) | 4.9165e+25 | 5.5602e+25 | 5.0870e+25 | 5.3834e+25 | 5.4637e+25 | 4.8574e+25 |
| ( 6.875, 7.125 ) | 3.4489e+25 | 3.9082e+25 | 3.5726e+25 | 3.7778e+25 | 3.8342e+25 | 3.4080e+25 |
| ( 7.125, 7.375 ) | 2.2031e+25 | 2.4946e+25 | 2.2806e+25 | 2.4123e+25 | 2.4504e+25 | 2.1791e+25 |
| ( 7.375, 7.625 ) | 1.4085e+25 | 1.5985e+25 | 1.4600e+25 | 1.5430e+25 | 1.5674e+25 | 1.3935e+25 |
| ( 7.625, 7.875 ) | 8.6630e+24 | 9.9248e+24 | 9.0282e+24 | 9.5053e+24 | 9.6625e+24 | 8.5850e+24 |
| ( 7.875, 8.125 ) | 5.0429e+24 | 5.7308e+24 | 5.2307e+24 | 5.5256e+24 | 5.6113e+24 | 4.9878e+24 |
| ( 8.125, 8.375 ) | 2.9606e+24 | 3.3351e+24 | 3.0552e+24 | 3.2391e+24 | 3.2861e+24 | 2.9225e+24 |
| ( 8.375, 8.625 ) | 1.7539e+24 | 1.9574e+24 | 1.8002e+24 | 1.9159e+24 | 1.9418e+24 | 1.7280e+24 |
| ( 8.625, 8.875 ) | 1.0489e+24 | 1.1593e+24 | 1.0705e+24 | 1.1439e+24 | 1.1584e+24 | 1.0315e+24 |
| ( 8.875, 9.125 ) | 6.3354e+23 | 6.9312e+23 | 6.4279e+23 | 6.8967e+23 | 6.9784e+23 | 6.2185e+23 |
| ( 9.125, 9.375 ) | 3.8648e+23 | 4.1849e+23 | 3.8980e+23 | 4.1997e+23 | 4.2465e+23 | 3.7870e+23 |
| ( 9.375, 9.625 ) | 2.3814e+23 | 2.5521e+23 | 2.3875e+23 | 2.5831e+23 | 2.6103e+23 | 2.3297e+23 |

TABLE XIV. Predicted reactor antineutrino energy spectrum from each nuclear reactor integrated over the data acquisition time of EH3 (2011/12/24-2013/11/27). Applicable to EH3-AD1, EH3-AD2, and EH3-AD3. The energy bins are presented as lower and upper bin edges.

| Energy [MeV] | Reactor 1 | Reactor 2 | Reactor 3 | Reactor 4 | Reactor 5 | Reactor 6 |
|---|---|---|---|---|---|---|
| ( 1.375, 1.625 ) | 4.3327e+27 | 4.2414e+27 | 4.0739e+27 | 4.4662e+27 | 4.3269e+27 | 4.3115e+27 |
| ( 1.625, 1.875 ) | 3.8592e+27 | 3.7783e+27 | 3.6263e+27 | 3.9711e+27 | 3.8490e+27 | 3.8350e+27 |
| ( 1.875, 2.125 ) | 3.2762e+27 | 3.2065e+27 | 3.0775e+27 | 3.3716e+27 | 3.2665e+27 | 3.2549e+27 |
| ( 2.125, 2.375 ) | 2.7817e+27 | 2.7214e+27 | 2.6121e+27 | 2.8630e+27 | 2.7724e+27 | 2.7628e+27 |
| ( 2.375, 2.625 ) | 2.2542e+27 | 2.2078e+27 | 2.1188e+27 | 2.3204e+27 | 2.2480e+27 | 2.2395e+27 |
| ( 2.625, 2.875 ) | 1.9007e+27 | 1.8596e+27 | 1.7854e+27 | 1.9579e+27 | 1.8946e+27 | 1.8879e+27 |
| ( 2.875, 3.125 ) | 1.5864e+27 | 1.5533e+27 | 1.4914e+27 | 1.6348e+27 | 1.5831e+27 | 1.5774e+27 |
| ( 3.125, 3.375 ) | 1.3119e+27 | 1.2883e+27 | 1.2367e+27 | 1.3521e+27 | 1.3122e+27 | 1.3063e+27 |
| ( 3.375, 3.625 ) | 1.0790e+27 | 1.0594e+27 | 1.0171e+27 | 1.1123e+27 | 1.0794e+27 | 1.0746e+27 |
| ( 3.625, 3.875 ) | 8.6506e+26 | 8.4954e+26 | 8.1553e+26 | 8.9167e+26 | 8.6562e+26 | 8.6173e+26 |
| ( 3.875, 4.125 ) | 6.8775e+26 | 6.7674e+26 | 6.4950e+26 | 7.0896e+26 | 6.8900e+26 | 6.8551e+26 |
| ( 4.125, 4.375 ) | 5.4392e+26 | 5.3474e+26 | 5.1325e+26 | 5.6068e+26 | 5.4463e+26 | 5.4201e+26 |
| ( 4.375, 4.625 ) | 4.1625e+26 | 4.1018e+26 | 3.9356e+26 | 4.2900e+26 | 4.1754e+26 | 4.1525e+26 |
| ( 4.625, 4.875 ) | 3.1843e+26 | 3.1419e+26 | 3.0141e+26 | 3.2814e+26 | 3.1976e+26 | 3.1789e+26 |
| ( 4.875, 5.125 ) | 2.4885e+26 | 2.4609e+26 | 2.3601e+26 | 2.5640e+26 | 2.5030e+26 | 2.4868e+26 |
| ( 5.125, 5.375 ) | 1.9516e+26 | 1.9302e+26 | 1.8510e+26 | 2.0106e+26 | 1.9635e+26 | 1.9508e+26 |
| ( 5.375, 5.625 ) | 1.4591e+26 | 1.4437e+26 | 1.3844e+26 | 1.5032e+26 | 1.4684e+26 | 1.4587e+26 |
| ( 5.625, 5.875 ) | 1.1512e+26 | 1.1386e+26 | 1.0918e+26 | 1.1856e+26 | 1.1589e+26 | 1.1515e+26 |
| ( 5.875, 6.125 ) | 8.4804e+25 | 8.4206e+25 | 8.0708e+25 | 8.7325e+25 | 8.5616e+25 | 8.4967e+25 |
| ( 6.125, 6.375 ) | 6.1230e+25 | 6.0989e+25 | 5.8424e+25 | 6.3009e+25 | 6.2007e+25 | 6.1486e+25 |
| ( 6.375, 6.625 ) | 4.6666e+25 | 4.6440e+25 | 4.4492e+25 | 4.8029e+25 | 4.7220e+25 | 4.6835e+25 |
| ( 6.625, 6.875 ) | 3.4757e+25 | 3.4583e+25 | 3.3130e+25 | 3.5764e+25 | 3.5177e+25 | 3.4893e+25 |
| ( 6.875, 7.125 ) | 2.4377e+25 | 2.4289e+25 | 2.3265e+25 | 2.5083e+25 | 2.4694e+25 | 2.4485e+25 |
| ( 7.125, 7.375 ) | 1.5574e+25 | 1.5507e+25 | 1.4852e+25 | 1.6019e+25 | 1.5779e+25 | 1.5649e+25 |
| ( 7.375, 7.625 ) | 9.9551e+24 | 9.9288e+24 | 9.5072e+24 | 1.0239e+25 | 1.0097e+25 | 1.0009e+25 |
| ( 7.625, 7.875 ) | 6.1169e+24 | 6.1424e+24 | 5.8763e+24 | 6.2898e+24 | 6.2343e+24 | 6.1679e+24 |
| ( 7.875, 8.125 ) | 3.5634e+24 | 3.5578e+24 | 3.4056e+24 | 3.6656e+24 | 3.6156e+24 | 3.5830e+24 |
| ( 8.125, 8.375 ) | 2.0937e+24 | 2.0775e+24 | 1.9898e+24 | 2.1545e+24 | 2.1143e+24 | 2.0990e+24 |
| ( 8.375, 8.625 ) | 1.2414e+24 | 1.2237e+24 | 1.1728e+24 | 1.2779e+24 | 1.2474e+24 | 1.2407e+24 |
| ( 8.625, 8.875 ) | 7.4316e+23 | 7.2751e+23 | 6.9771e+23 | 7.6524e+23 | 7.4294e+23 | 7.4042e+23 |
| ( 8.875, 9.125 ) | 4.4928e+23 | 4.3669e+23 | 4.1910e+23 | 4.6276e+23 | 4.4682e+23 | 4.4623e+23 |
| ( 9.125, 9.375 ) | 2.7435e+23 | 2.6473e+23 | 2.5425e+23 | 2.8264e+23 | 2.7143e+23 | 2.7165e+23 |
| ( 9.375, 9.625 ) | 1.6922e+23 | 1.6210e+23 | 1.5579e+23 | 1.7436e+23 | 1.6656e+23 | 1.6705e+23 |

TABLE XV. Predicted reactor antineutrino energy spectrum from each nuclear reactor integrated over the data acquisition time of EH3 during the 8-AD period (2012/10/19-2013/11/27). Applicable to EH3-AD4. The energy bins are presented as lower and upper bin edges.
